# Supplementary material for: SMaCk: Efficient Instruction Cache Attacks via Self-Modifying Code Conflicts
Source: arXiv:2502.05429 source file (2025-02-08)
Supplement: Supplementary file 1 [file Appendix_AE.tex]

% LaTeX template for Artifact Evaluation V20240722
%
% Prepared by Grigori Fursin with contributions from Bruce Childers,
%   Michael Heroux, Michela Taufer and other colleagues.
%
% See examples of this Artifact Appendix in
%  * ASPLOS'24 "PyTorch 2: Faster Machine Learning Through Dynamic Python Bytecode Transformation and Graph Compilation": 
%      https://dl.acm.org/doi/10.1145/3620665.3640366
%  * SC'17 paper: https://dl.acm.org/citation.cfm?id=3126948
%  * CGO'17 paper: https://www.cl.cam.ac.uk/~sa614/papers/Software-Prefetching-CGO2017.pdf
%  * ACM ReQuEST-ASPLOS'18 paper: https://dl.acm.org/citation.cfm?doid=3229762.3229763
%
% (C)opyright 2014-2024 cTuning.org
%
% CC BY 4.0 license
%

\appendix
\section{Artifact Appendix}

%%%%%%%%%%%%%%%%%%%%%%%%%%%%%%%%%%%%%%%%%%%%%%%%%%%%%%%%%%%%%%%%%%%%%
\subsection{Abstract}
SMaCk provides a comprehensive set of artifacts to reproduce the key findings of our study. Our artifact package includes the prototype implementation of 8 distinct Prime and Probe attacks and 8 distinct Spectre attacks utilizing SMC behavior. Specifically, Table~\ref{table:Spectre_attacks} illustrates the application across 10 different microarchitectures through various strategies. These artifacts enable researchers to validate our attack methodologies and extend the study to additional microarchitectures. 

\subsection{Artifact check-list (meta-information)}

{\small
\begin{itemize}
  \item {\bf Algorithm:} Prime+iProbe, ISpectre
  \item {\bf Program:} Attack implementations, data collection scripts
  \item {\bf Compilation:} gcc 
  \item {\bf Binary:} Executable binaries for attack tools
  \item {\bf Data set:} Cache timing measurements
  \item {\bf Run-time environment:} Ubuntu
20.04.6 LTS
  \item {\bf Hardware:}  Intel Cascade Lake, Intel Comet Lake, AMD Ryzen 5 and listed Table~\ref{table:Spectre_attacks}
  \item {\bf Run-time state:} Configurations for shared physical cores with SMT enabled
  \item {\bf Output:} CSV files and PNG graph
  \item {\bf Experiments:} Time difference measurement, Prime and Probe attacks, Spectre attacks
  \item {\bf How much disk space required (approximately)?: } 5 GB
  \item {\bf How much time is needed to prepare workflow (approximately)?: } 2 hours 
  \item {\bf How much time is needed to complete experiments (approximately)?: } 5 hours 
  \item {\bf Publicly available?: } Yes, post-embargo. \url{https://github.com/hunie-son/SMaCk.git}
  \item {\bf Code licenses (if publicly available)?: } MIT License
  \item {\bf Workflow automation framework used?: } Makefile, Bash scripts
\end{itemize}
}

%%%%%%%%%%%%%%%%%%%%%%%%%%%%%%%%%%%%%%%%%%%%%%%%%%%%%%%%%%%%%%%%%%%%%
\subsection{Description}\label{appendix:Description}

\subsubsection{How to access}
The SMaCk artifact can be downloaded from the GitHub repository. Researchers can download the complete toolkit by visiting \url{https://github.com/hunie-son/SMaCk}.
Detailed instructions for accessing, setting up, and utilizing the artifacts to replicate the experiments and results presented in our paper are provided in the \texttt{README.md} file within the repository.

\subsubsection{Hardware dependencies}
SMaCk requires specific hardware configurations to effectively perform and evaluate L1i cache attacks. The toolkit has been evaluated on 10 distinct x86 microarchitectures, including Intel Cascade Lake, Tiger Lake, Comet Lake, and AMD Ryzen (Table~\ref{table:Spectre_attacks}). It is essential to have access to processors that support Simultaneous Multithreading (SMT), as this feature is crucial for creating and measuring SMC conflicts.

\subsubsection{Software dependencies}
The SMaCk toolkit is designed to run on Ubuntu 20.04.6 LTS and requires several software dependencies to function correctly. Essential tools include a C/C++ compiler (e.g., GCC, g++). MATLAB R2021 is also utilized for data visualization purposes. Moreover, tools such as \texttt{taskset} for CPU core affinity management is necessary. 

%%%%%%%%%%%%%%%%%%%%%%%%%%%%%%%%%%%%%%%%%%%%%%%%%%%%%%%%%%%%%%%%%%%%%
\subsection{Installation}
To install and set up the SMaCk toolkit, follow the steps outlined below. Ensure that your system meets the hardware and software dependencies specified in Section~\ref{appendix:Description}.

\noindent\textbf{Step 1: Clone repository}\\
{\em 
\noindent git clone \url{https://github.com/hunie-son/SMaCk.git}\\
cd SMaCk}

\noindent\textbf{Step 2: Navigate to the cache timing analysis directory and compile the toolkit}\\
{\em 
\noindent cd SMaCk\_cachetime\\
make}

\noindent\textbf{Step 3: Execute}
{\em 
\noindent taskset -c <core\#> ./smack\_cachetime > \{name\}\_csv\\
}

\noindent Similarly, verify that the executable mastik\_cachetime is present. Proceed to compile the attack variants by navigating to their respective directories and running make:\\

{\em 
\noindent cd ../SMaCk\_PNP\\
\noindent python3 prime\_probe\_gen.py <function\_name> i
\\make\\

\noindent cd ../Mastik\_PNP\\
make\\

\noindent cd ../SMaCk\_ISpectre\\
make\\
}

\noindent Ensure that all attack binaries (pnp\_attack, mastik\_pnp, smack\_ispectre) are successfully compiled without error.

%%%%%%%%%%%%%%%%%%%%%%%%%%%%%%%%%%%%%%%%%%%%%%%%%%%%%%%%%%%%%%%%%%%%%
\subsection{Experiment workflow}
The experiment workflow for SMaCk involves several steps. Starting with data collection on target microarchitecture and data visualization.

\noindent\textbf{Data Collection for Target microarchitecture:} Collecting cache timing data for target microarchitecture is the initial step of our workflow. Navigate to the cache timing analysis directory and execute the \texttt{smack\_cachetime} binary with appropriate CPU core affinity.\\
\\
{\em 
\noindent cd SMaCk\_cachetime\\
make\\
taskset -c <core\_number> ./smack\_cacketime > <microarchitecture\_name>\_smack\_cachetime.csv \\
}

\noindent Collect data using the Mastik Toolkit~\cite{yarom2016mastik} for a baseline comparison.\\
\\
{\em 
\noindent cd Mastik\_cachetime\\
make\\
taskset -c <core\_number> ./mastik\_cacketime > <microarchitecture\_name>\_mastik\_cachetime.csv \\
}

\noindent Use MATLAB code to visualize the collected data. The researcher needs to ensure that the MATLAB code is correctly configured to process the generated CSV files.\\
\\
{\em 
\noindent cache\_draw.m\\

\noindent cache\_draw\_intel.m\\
}

\noindent\textbf{Perform Prime and IProbe Attacks:} Execute Prime and IProbe attacks to generate cache eviction data. The Prime and Probe attack variants attack by navigating the attack binary. Various Probe function names are listed in Figure~\ref{fig:CPUcycleTime_cascade}.\\
\\
{\em 
\noindent cd SMaCk\_PNP\\
python3 prime\_probe\_gen.py <function\_name> i \\
make\\
taskset -c <core\_number> ./pnp\_attack <target\_cache\_set> <delay\_cycle> <samples> \\
}

\noindent Performing Prime using the Mastik Toolkit [52] for a baseline comparison.\\
\\
{\em 
\noindent cd Mastik\_PNP\\
make\\
taskset -c <core\_number> ./mastik\_attack <target\_cache\_set> <delay\_cycle> <samples> \\
}

\noindent\textbf{Perform ISpectre Attacks:} Execute Spectre attacks utilizing SMC behavior to exploit speculative execution vulnerabilities.\\
\\
{\em 
\noindent cd SMaCk\_ISpectre\\
make\\
taskset -c <core\_number> ./smack\_ispectre <Function\_name> <Iteration> <Anomaly> \\
}

\noindent For example: 
{\em 
\noindent taskset -c 0 ./smack\_ispectre flush 1000 500 \\
}

%%%%%%%%%%%%%%%%%%%%%%%%%%%%%%%%%%%%%%%%%%%%%%%%%%%%%%%%%%%%%%%%%%%%%
\subsection{Evaluation and expected results}
Upon successful installation and execution of the SMaCk toolkit, researchers can reproduce the key results detailed in our paper.
The evaluation focuses on demonstrating the effectiveness of SMaCk in performing L1i cache attacks and the leak of sensitive information.

\noindent\textbf{Cache Timing Analysis:} Researcher should observe distinct timing discrepancies between L1d, L1i, L2, LLC and DRAM for various Probe strategies as depicted in Figure~\ref{fig:CPUcycleTime_cascade}. The MATLAB code will generate a visualization plot illustrating the impact of SMC conflicts on cache timing and highlighting the measurable difference.

\noindent\textbf{Prime+iProbe Attack:} Executing Prime and IProbe attacks utilizing SMaCk should result in high bandwidth covert channels with low error rates. This attack is outstanding to baseline results obtained using Mastik Toolkit~\cite{yarom2016mastik}. Researchers will successfully evict target cache sets with effective performing prime and probe attacks to leak information leakage. 

\noindent\textbf{ISpectre Attack:} SMaCk offers various types of ISpectre attacks, which demonstrates the ability to exploit speculative execution to leak secret key bits. Researchers can expect high success rates in leaking secret bytes. These attacks are feasible across 10 different microarchitectures through various strategies, as shown in Table~\ref{table:Spectre_attacks}.

%Submission, reviewing and badging methodology:
\begin{comment}
    
\begin{itemize}
  \item \url{https://www.acm.org/publications/policies/artifact-review-and-badging-current}
  \item \url{https://cTuning.org/ae}
\end{itemize}
\end{comment}
