# Supplementary material for: SMaCk: Efficient Instruction Cache Attacks via Self-Modifying Code Conflicts
Source: arXiv:2502.05429 source file (2025-02-08)
Supplement: Supplementary file 2 [file Appendix_old.tex]

\section{Appendix}

\begin{comment}
\subsection{Code Snippets for Cache State Preparations}\label{sec:cache_code}

\lstset{style=mystyle}
\begin{lstlisting}[caption={Different Cache State Preparation Codes used in Timing Histogram Preparation},label=lst:memory_prepare]
big_16mb:
    .space 16 * 1024 * 1024, 0xcc
    
.text
.align 0x1000
.global evict_n
evict_n:
    push %r11
    lea big_16mb, %r11
evict_n_label:
    mov (%r11, %rdi, 1), %rax
    sub $64, %rdi
    jnz evict_n_label
    mfence
    pop %r11
    ret

prepare_L1d(){
    mov (%rdi), %rax
    mfence
}

prepare_L3()
{
    mov (%rdi), %rax
    evict_n(1024*32)
    mfence
}

prepare_DRAM()
{
    flush_time((uint64_t *)oracle_code_page)
    mfence
}

\end{lstlisting}

%%%%%%%%%%%%%%%%%%%%%%%%%%%%%%%%%%%%%%%%%%%%%%%%%%%%%%%%%%%%%
\end{comment}
%\newpage
\begin{comment}
\subsection{Intel Tiger Lake}\label{sec:Tigerlake}

\begin{figure}[ht]
    \centering
    {
    \includegraphics[width=\linewidth]{Source/Sections/Figures/cacheops_intel_tigerlake_v3.png}
    }
    \caption{CPU cycle time difference with different Probe strategies on Intel Tiger Lake microarchitecture.}
    \label{fig:CPUcycleTime_tigerlake}
    %\vspace{-6mm}
\end{figure}

\newpage
\subsection{AMD Ryzen 5}\label{sec:AMD}

\begin{figure}[ht]
    \centering
    {
    \includegraphics[width=\linewidth]{Source/Sections/Figures/cacheops_amd_ryzen_v2.png}
    }
    \caption{CPU cycle time difference with different Probe strategies on AMD Ryzen 5 microarchitecture.}
    \label{fig:CPUcycleTime_amd_ryzen}
    %\vspace{-6mm}
\end{figure}
\end{comment}
\begin{comment}
\subsection{AMD EPYC}\label{sec:AMD}

\begin{figure}[ht!]
    \centering
    {
    \includegraphics[width=\linewidth]{Source/Sections/Figures/cacheops_amd_epyc.png}
    }
    \caption{CPU cycle time difference with different Probe strategies on AMD Ryzen 5 microarchitecture.}
    \label{fig:CPUcycleTime_amd_epyc}
    %\vspace{-6mm}
\end{figure}

%\newpage

    
\subsection{Intel Ice Lake}\label{sec:Icelake}

\begin{figure}[ht!]
    \centering
    {
    \includegraphics[width=\linewidth]{Source/Sections/Figures/cacheops_icelake_non.png}
    }
    \caption{CPU cycle time difference with different Probe strategies on Ice Lake microarchitecture.}
    \label{fig:CPUcycleTime_icelake}
    %\vspace{-6mm}
\end{figure}

\newpage
\subsection{Intel Broadwell}\label{sec:Broadwell}
\begin{figure}[ht!]
    \centering
    {
    \includegraphics[width=\linewidth]{Source/Sections/Figures/cacheops_broadwell.png}
    }
    \caption{CPU cycle time difference with different Probe strategies on Broadwell microarchitecture.}
    \label{fig:CPUcycleTime_broadwell}
    %\vspace{-6mm}
\end{figure}
\end{comment}

%%%%%%%%%%%%%%%%%%%%%%%%%%%%%%%%%%%%%%%%%%%%%%%%%%%%%%%%%


%\newpage
\onecolumn
\FloatBarrier
\subsection{PAPI counter option}\label{sec:papi_counters}
\begin{table*}[ht!]
\centering
\caption{SMC related PAPI counter option for Reverse Engineering }
\setlength{\tabcolsep}{5pt}
\scalebox{0.58}{
\begin{tabular}{l|l|l}
\hline
\textbf{Type}                    & \textbf{Counter Name}                                        & \textbf{Description}                                                                                                                                   \\ \hline
\multirow{15}{*}{\textbf{Intel}} & MACHINE\_CLEARS.COUNT                               & Number of machine clears of any type                                                                                                          \\ 
                        & MACHINE\_CLEARS.SMC                                 & Number of SMC Machine Clears detected                                                                                                         \\ 
                        & INT\_MISC.RECOVERY\_CYCLES                          & Cycles waiting for the checkpoints in Resource Allocation Table to be recovered after Nuke                                                    \\  
                        & INT\_MISC.RECOVERY\_CYCLES\_ANY                     & Core cycles the allocator was stalled due to recovery from earlier clear events for any thread running on the physical core                   \\  
                        & INT\_MISC.CLEAR\_RESTEER\_CYCLES                    & The issue-stage waiting for front-end to fetch from resteered path following branch misprediction/machine clear \\ 
                        & CYCLE\_ACTIVITY                                     & Stalled cycle                                                                                                                                 \\  
                        & CYCLE\_ACTIVITY.CYCLES\_MEM\_ANY                    & Cycles when memory subsystem has at least one outstanding load                                                                                \\  
                        & CYCLE\_ACTIVITY.STALLS\_MEM\_ANY                    & Execution stalls while at least one demand load is outstanding in the memory subsystem                                                        \\  
                        & CYCLE\_ACTIVITY.STALLS\_TOTAL                       & Total execution stalls in cycles                                                                                                              \\  
                        & ICACHE\_16B.IFDATA\_STALL                           & Cycles where a code fetch is stalled due to L1 instruction cache miss                                                                         \\  
                        & ICACHE\_64B.IFTAG\_HIT                              & Number of instruction fetch tag lookups that hit in the instruction cache (L1I). Counts at 64-byte cache-line granularity                     \\  
                           
                        & RESOURCE\_STALLS.ANY                                & Cycles Allocation is stalled due to Resource Related reason                                                                                   \\  
                        & RESOURCE\_STALLS.ALL                                & Cycles Allocation is stalled due to Resource Related reason \\
                         & FRONTEND\_RETIRED.IDQ\_4\_BUBBLES.fe\_thres=20                                & Retired instructions after an interval where the front-end did not deliver any uops (4 bubbles) for a period determined by the fe\_thres and not interrupted by a back-end stall \\
                          & PARTIAL\_RAT\_STALLS.SCOREBOARD & RAT stalls: Count core cycles where the pipeline is stalled due to serialization operations 
                                                                                                                                              \\ \hline
\multirow{2}{*}{\textbf{AMD}}    & INSTRUCTION\_PIPE\_STALL .IC\_STALL\_ANY            & IC pipe was stalled during this clock cycle for any reason                                                                                    \\  
                        & INSTRUCTION\_PIPE\_STALL.IC\_STALL\_BACK\_PRESSURE & IC PIPE was stalled during this clock cycle(IC to OC fetches) due to the back pressure                                                        \\ 
                        & CYCLES\_WITH\_FILL\_PENDING\_FROM\_L2:L2\_FILL\_BUSY & Total cycles spent with one or more fill requests in flight from L2                                                   \\
                        & perf::PERF\_COUNT\_HW\_CACHE\_MISSES & PERF\_COUNT\_HW\_CACHE\_MISSES                                                  \\
                        
                        \hline
\end{tabular}
}
\label{tab:counters}
\end{table*}
\FloatBarrier

    

    

%%%%%%%%%%%%%%%%%%%%%%%%%%%%%%%%%%%%%%%%%%%%%%%%%%%%%%%%%%%%%%%%%
%\newpage

\FloatBarrier
\subsection{Keystroke result}\label{sec:keystroke_result}
\begin{table*}[ht!]
\centering
\caption{Keystroke Word classification utilizing kNN for Original dataset\cite{killourhy2012free}, \texttt{Prime+iFlush}, \texttt{Prime+iStore}, \texttt{Prime+iLock} and \texttt{Prime+iClwb} attack}
\setlength{\tabcolsep}{5pt}
\scalebox{0.75}{
\begin{tabular}{cccc|ccc|ccc|ccc|ccc|ccc} & & &  & \multicolumn{3}{c|}{\textbf{Original Accuracy}}  & \multicolumn{3}{c|}{\textbf{Prime+iFlush Accuracy}} & \multicolumn{3}{c|}{\textbf{Prime+iStore Accuracy}} & \multicolumn{3}{c|}{\textbf{Prime+iLock Accuracy}} & \multicolumn{3}{c}{\textbf{Prime+iClwb Accuracy}}         \\
\textbf{subject}  & \textbf{\begin{tabular}[c]{@{}c@{}}Training\\ set\end{tabular}} & \textbf{\begin{tabular}[c]{@{}c@{}}Test \\ set\end{tabular}} & \textbf{\begin{tabular}[c]{@{}c@{}}Unique\\ word\end{tabular}} & \textbf{Test}  & \textbf{top-5} & \textbf{top-10} & \textbf{Test}  & \textbf{top-5} & \textbf{top-10}& \textbf{Test}  & \textbf{top-5} & \textbf{top-10} & \textbf{Test}  & \textbf{top-5} & \textbf{top-10} & \textbf{Test}  & \textbf{top-5} & \textbf{top-10}  \\ \hline
s019 & 695 & 263 & 181  & 33.46  & 55.51 & 65.01& 32.32 &55.51 & 66.92& 31.56& 54.37 & 66.16 &31.94 &53.99 &64.26& 32.70 & 53.23& 66.16\\
s021  & 613 & 236  & 154& 29.66 & 51.27 & 64.83 &25.85 &55.08 & 70.76 & 27.12  & 55.51 & 70.76 &25.00 &52.97 &66.53 & 26.69 &54.66 & 69.49\\
s027 & 543& 210& 132 & 32.38 & 60.00 & 69.52 & 32.86 &58.57 & 76.19  & 31.91 & 59.52& 77.14 &31.43 & 55.71&72.38 & 31.90 &57.14 & 75.71\\
s033  & 771 & 292 & 190 & 31.50& 60.61 & 69.52  & 31.85 &56.51 & 70.21  & 32.19  & 56.51  & 69.52 &31.51 &54.79 &69.18 & 31.51 &55.48 & 70.21\\
s039    & 643    & 242 & 170 & 33.05 & 63.23 & 72.72 & 26.86 &51.24 & 67.77  & 27.69 & 53.31 & 68.18 &28.93&49.17 &65.70 & 28.51 &51.24 & 67.36\\ \hline
s040 & 607 & 231 & 142  & 32.03 & 52.81 & 68.39 & 35.50 &57.58 & 65.37  & 35.93  & 58.01  & 66.23  &33.33 &53.68 & 61.90& 34.63 &56.71 & 64.94\\
s043 & 808 & 332& 181  & 34.03  & 59.93    & 71.08  & 34.94 &67.47 & 77.11  & 34.64   & 66.87   & 77.41 &34.94&64.76 &76.20 & 34.64 &66.87 & 76.20\\
s046  & 750 & 299  & 172   & 29.76 & 58.86 & 66.55 &35.79 &64.21 & 74.25  & 35.45   & 64.55    & 74.92 &36.79 &63.55&74.58 &34.78 &63.88 & 75.59\\
s062  & 676  & 254  & 176 & 23.62 & 50.78 & 62.20 & 30.71 &58.27 & 70.47 & 29.53 & 57.09 & 72.44 &29.92 &57.87 &68.50 &28.74 &57.87 & 70.08\\
s063 & 610 & 224   & 157& 20.53 & 50.89  & 63.39 & 27.23 &53.57 & 66.07 & 29.02 & 54.91  & 66.07 &29.02 &54.46 & 65.62& 26.34 &52.68 & 66.52\\ \hline
s067& 574   & 223  & 138    & 32.73 & 61.43 & 72.19 & 33.18 &62.33 & 76.23  &33.18& 60.99& 77.13 &32.74 &58.74 &73.09 & 32.74 &60.99 & 76.68\\
s070   & 600   & 231  & 151& 27.27  & 58.00 & 67.09   &  28.14 &59.31 & 75.32  &  29.87 & 60.61& 76.19 &29.00 & 60.17&75.32 &31.17 &61.04 & 76.62\\
 s071   & 892 & 359& 197   & 26.46 & 52.08 & 64.34& 28.97 &57.10 & 72.42  & 28.69 & 57.10& 71.87&29.53 &55.99 &69.36 & 28.97 &57.38 & 71.31 \\
s085  & 580  & 234    & 137  & 29.05    & 60.68    & 72.22    & 33.76 &65.38 & 75.64  & 32.91    & 66.23    & 76.92 &32.91 &63.25 &75.64 &32.48 &64.96 & 76.07 \\
s087 & 668     & 254  & 166   & 35.58   & 64.96    & 72.83  & 37.40 &65.35 & 76.77  &38.19   & 66.54     & 77.95  &36.22 &62.60&75.59 & 37.40 &65.75 & 75.59\\ \hline
s089   & 614  & 240  & 154   & 28.75    & 55.83   & 68.75 &  24.58 &62.50 & 74.17 & 24.17 & 60.0 & 73.33 &25.00 &58.75 & 73.75& 24.58 &59.17 & 72.92\\
s091  & 778     & 313   & 174  & 21.72  & 47.28   & 62.30 & 22.04 &46.01 & 62.62  & 22.36 & 46.33 & 62.94 &20.45 &46.33 & 61.34&20.77 &46.01 & 62.30\\
s092 & 646  & 254  & 154 & 26.37   & 56.69   & 70.86 & 29.53 &62.60 & 76.77  &29.13 & 62.99 & 77.17 &28.35 &61.02 &75.98 &28.74 &64.57 & 76.38 \\
s093  & 616 & 239  & 145   & 30.54  & 58.57   & 64.85   & 31.80 &59.00 & 68.62  & 33.05 & 63.60 & 69.87 &32.64& 59.00&68.20 &30.96 &60.67 & 68.20\\
s094   & 648   & 259   & 151    & 28.18  & 58.30    & 68.72 & 35.14 &60.23 & 71.43 &35.52  & 59.07 & 72.97 &33.59 & 59.07& 70.66&35.14 &58.30 & 71.81\\ \hline
{ \textbf{Avergae}} & \textbf{666.6}   & \textbf{259.45}  & \textbf{161.1} & \textbf{29.48} & \textbf{56.88} & \textbf{67.87}  & \textbf{30.92} & \textbf{58.89} & \textbf{71.76} & \textbf{31.11} & \textbf{59.21} & \textbf{72.26} & \textbf{30.66} & \textbf{57.29} & \textbf{70.19} & \textbf{30.67} & \textbf{58.43} & \textbf{71.51} \\ \hline
\end{tabular}
}
\label{table:Keystroke_result}
\end{table*}

\FloatBarrier

\twocolumn
\FloatBarrier
\begin{figure}[ht]
    \centering
    {
    \includegraphics[width=\linewidth]{Source/Sections/Figures/KSResult_uncompromising_meg.png}
    }
    \caption{Keystroke detection example utilizing Prime+IStore attack. Focused on the keypress activity for setting sliding window size}
    \label{fig:Keystroke_uncompromising_meg}
\end{figure} 
\FloatBarrier


%%%%%%%%%%%%%%%%%%%%%%%%%%%%%%%%%%%%%%%%%%%%%%%%%%%%%%

\FloatBarrier


\subsection{Dynamic detection tool result}\label{sec:Dynamic_detection_tool_result}

A more sophisticated detection tool can utilize the \texttt{cycle\_activity.stalls\_total} counter with high accuracy and F-score. This counter is helpful because SMC behavior flushes the pipeline in the L1i cache, causing the stall cycle.
Based on our observations with 9 different counters, we select the top 3 counters to create the dynamic detection tool. We achieve 97.18\% test accuracy F-score of 0.9391 and FPR of 1.67\% on \texttt{Prime+iProbe} type attack and test accuracy of 97.37\% and F-score of 0.9447 with an FPR of 2.34\% on \texttt{Flush+iReload} attacks utilizing dynamic detection tool. Note that the value of the machine\_clear-related counter is relatively higher on the \texttt{Prime+iProbe} type attack rather than the \texttt{Flush+iReload} attacks (Figure~\ref{fig:detection_result}). This is because our \texttt{Prime+iProbe} fills the L1i cache and invalidates 8 ways of the L1i cache line, which creates SMC behavior on all 8 ways of the cache line. However, \texttt{ISpectre} attacks only create the SMC behavior on the secret bytes range and no SMC conflict for the wrong secret byte candidates. Overall, we achieve only 0.9\% performance overhead when a single counter is monitored with 100 ms resolution.
%}


\begin{table}[h]
\centering
\caption{Counter selection for SMC based \texttt{Prime+iProbe} attack}
\setlength{\tabcolsep}{7pt}
\scalebox{1}{
\begin{tabular}{|l|ccc|}
\hline
\multirow{2}{*}{\textbf{Counter}} & \multicolumn{3}{c|}{\textbf{F-score}}                                              \\ \cline{2-4} 
                                  & \multicolumn{1}{c|}{\textbf{SVM}} & \multicolumn{1}{c|}{\textbf{RF}} & \textbf{DF} \\ \hline
br-misp-retired-all-branches      & \multicolumn{1}{c|}{0.0000}       & \multicolumn{1}{c|}{0.8350}      & 0.8350      \\ \hline
br-inst-retired-all-branches      & \multicolumn{1}{c|}{0.4072}       & \multicolumn{1}{c|}{0.7692}      & 0.7692      \\ \hline
longest-lat-cache-miss            & \multicolumn{1}{c|}{0.0000}       & \multicolumn{1}{c|}{0.7656}      &  0.7656      \\ \hline
cache-references                  & \multicolumn{1}{c|}{0.0000}       & \multicolumn{1}{c|}{0.7755}      & 0.7755      \\ \hline
cache-misses                       & \multicolumn{1}{c|}{0.0000}       & \multicolumn{1}{c|}{0.8000}      & 0.8000      \\ \hline
\textbf{cycle-activity-stalls-total}       & \multicolumn{1}{c|}{0.8539}       & \multicolumn{1}{c|}{ 0.9170}      &  0.9170      \\ \hline
\textbf{machine-clears-count}              & \multicolumn{1}{c|}{0.9825}       & \multicolumn{1}{c|}{0.9870}      & 0.9870      \\ \hline
\textbf{machine-clears-smc}                & \multicolumn{1}{c|}{0.9802}       & \multicolumn{1}{c|}{0.9659}      & 0.9659      \\ \hline
L1-icache-load-misses                & \multicolumn{1}{c|}{0.7287}       & \multicolumn{1}{c|}{0.7644}      & 0.7644      \\ \hline
\end{tabular}
}
\label{table:DynamicDetectionTool_pnp}
\end{table}


\newpage
\begin{table}[h]
\centering
\caption{Counter selection for SMC based \texttt{iSpectre} attack}
\setlength{\tabcolsep}{7pt}
\scalebox{1}{
\begin{tabular}{|l|ccc|}
\hline
\multirow{2}{*}{\textbf{Counter}} & \multicolumn{3}{c|}{\textbf{F-score}}                                              \\ \cline{2-4} 
                                  & \multicolumn{1}{c|}{\textbf{SVM}} & \multicolumn{1}{c|}{\textbf{RF}} & \textbf{DF} \\ \hline
br-misp-retired-all-branches      & \multicolumn{1}{c|}{0.0000}       & \multicolumn{1}{c|}{0.9399}      & 0.9399      \\ \hline
br-inst-retired-all-branches      & \multicolumn{1}{c|}{0.0000}       & \multicolumn{1}{c|}{0.8783}      & 0.8783      \\ \hline
\textbf{longest-lat-cache-miss}            & \multicolumn{1}{c|}{0.0000}       & \multicolumn{1}{c|}{0.9100}      & 0.9100      \\ \hline
cache-references                  & \multicolumn{1}{c|}{0.0000}       & \multicolumn{1}{c|}{0.7789}      & 0.7789      \\ \hline
cache-misses                       & \multicolumn{1}{c|}{0.0000}       & \multicolumn{1}{c|}{0.8842}      & 0.8842      \\ \hline
\textbf{cycle-activity-stalls-total}       & \multicolumn{1}{c|}{0.9135}       & \multicolumn{1}{c|}{0.9375}      & 0.9375      \\ \hline
\textbf{machine-clears-count}              & \multicolumn{1}{c|}{0.8063}       & \multicolumn{1}{c|}{0.8352}      & 0.8352      \\ \hline
\textbf{machine-clears-smc}                & \multicolumn{1}{c|}{0.9645}       & \multicolumn{1}{c|}{1.0000}      & 1.0000      \\ \hline
L1-icache-load-misses                & \multicolumn{1}{c|}{0.0000}       & \multicolumn{1}{c|}{0.4103}      & 0.4103      \\ \hline

\end{tabular}
}
\label{table:DynamicDetectionTool_ispectre}
\end{table}

\begin{table}[h]
\centering
\caption{Counter selection for both SMC based \texttt{Prime+iProbe} and \texttt{iSpectre} attack}
\setlength{\tabcolsep}{7pt}
\scalebox{1}{
\begin{tabular}{|l|ccc|}
\hline
\multirow{2}{*}{\textbf{Counter}} & \multicolumn{3}{c|}{\textbf{F-score}}                                              \\ \cline{2-4} 
                                  & \multicolumn{1}{c|}{\textbf{SVM}} & \multicolumn{1}{c|}{\textbf{RF}} & \textbf{DF} \\ \hline
br-misp-retired-all-branches      & \multicolumn{1}{c|}{0.0000}       & \multicolumn{1}{c|}{0.9034}      & 0.9034      \\ \hline
br-inst-retired-all-branches      & \multicolumn{1}{c|}{0.0000}       & \multicolumn{1}{c|}{0.8519}      & 0.8519      \\ \hline
longest-lat-cache-miss            & \multicolumn{1}{c|}{0.8111}       & \multicolumn{1}{c|}{0.8549}      & 0.8549      \\ \hline
cache-references                  & \multicolumn{1}{c|}{0.0000}       & \multicolumn{1}{c|}{0.8276}      & 0.8276      \\ \hline
cache-misses                       & \multicolumn{1}{c|}{0.6338}       & \multicolumn{1}{c|}{0.8454}      & 0.8454      \\ \hline
\textbf{cycle-activity-stalls-total}       & \multicolumn{1}{c|}{0.8899}       & \multicolumn{1}{c|}{0.9286}      & 0.9286      \\ \hline
\textbf{machine-clears-count}              & \multicolumn{1}{c|}{0.8974}       & \multicolumn{1}{c|}{0.8941}      & 0.8969      \\ \hline
\textbf{machine-clears-smc}                & \multicolumn{1}{c|}{0.7023}       & \multicolumn{1}{c|}{0.9792}      & 0.9792      \\ \hline
L1-icache-load-misses                & \multicolumn{1}{c|}{0.5491}       & \multicolumn{1}{c|}{0.5642}      & 0.5642      \\ \hline

\end{tabular}
}
\label{table:DynamicDetectionTool_pnip_ispectre}
\end{table}












\FloatBarrier
\begin{comment}
=== Scenario 1 Benign & PNiP ===
  Counter: longest-lat-cache-miss, Model: SVM, Accuracy: 0.7799, F1-Score: 0.0000
  Counter: longest-lat-cache-miss, Model: Decision Tree, Accuracy: 0.8953, F1-Score: 0.7656
  Counter: longest-lat-cache-miss, Model: Random Forest, Accuracy: 0.8953, F1-Score: 0.7656
  Counter: br-misp-retired-all-branches, Model: SVM, Accuracy: 0.7799, F1-Score: 0.0000
  Counter: br-misp-retired-all-branches, Model: Decision Tree, Accuracy: 0.9274, F1-Score: 0.8350
  Counter: br-misp-retired-all-branches, Model: Random Forest, Accuracy: 0.9274, F1-Score: 0.8350
  Counter: br-inst-retired-all-branches, Model: SVM, Accuracy: 0.7799, F1-Score: 0.0000
  Counter: br-inst-retired-all-branches, Model: Decision Tree, Accuracy: 0.8974, F1-Score: 0.7692
  Counter: br-inst-retired-all-branches, Model: Random Forest, Accuracy: 0.8974, F1-Score: 0.7692
  Counter: cycle-activity-stalls-total, Model: SVM, Accuracy: 0.9167, F1-Score: 0.8539
  Counter: cycle-activity-stalls-total, Model: Decision Tree, Accuracy: 0.9594, F1-Score: 0.9170
  Counter: cycle-activity-stalls-total, Model: Random Forest, Accuracy: 0.9594, F1-Score: 0.9170
  Counter: cache-misses, Model: SVM, Accuracy: 0.7799, F1-Score: 0.0000
  Counter: cache-misses, Model: Decision Tree, Accuracy: 0.9060, F1-Score: 0.8000
  Counter: cache-misses, Model: Random Forest, Accuracy: 0.9060, F1-Score: 0.8000
  Counter: L1-icache-load-misses, Model: SVM, Accuracy: 0.8562, F1-Score: 0.7287
  Counter: L1-icache-load-misses, Model: Decision Tree, Accuracy: 0.8863, F1-Score: 0.7644
  Counter: L1-icache-load-misses, Model: Random Forest, Accuracy: 0.8863, F1-Score: 0.7644
  Counter: machine-clears-smc, Model: SVM, Accuracy: 0.9915, F1-Score: 0.9802
  Counter: machine-clears-smc, Model: Decision Tree, Accuracy: 0.9850, F1-Score: 0.9659
  Counter: machine-clears-smc, Model: Random Forest, Accuracy: 0.9850, F1-Score: 0.9659
  Counter: machine-clears-count, Model: SVM, Accuracy: 0.9915, F1-Score: 0.9825
  Counter: machine-clears-count, Model: Decision Tree, Accuracy: 0.9936, F1-Score: 0.9870
  Counter: machine-clears-count, Model: Random Forest, Accuracy: 0.9936, F1-Score: 0.9870
  Counter: cache-references, Model: SVM, Accuracy: 0.7799, F1-Score: 0.0000
  Counter: cache-references, Model: Decision Tree, Accuracy: 0.9060, F1-Score: 0.7755
  Counter: cache-references, Model: Random Forest, Accuracy: 0.9081, F1-Score: 0.7795

=== Scenario 2 Benign & iSpectre ===
  Counter: longest-lat-cache-miss, Model: SVM, Accuracy: 0.7889, F1-Score: 0.0000
  Counter: longest-lat-cache-miss, Model: Decision Tree, Accuracy: 0.9600, F1-Score: 0.9100
  Counter: longest-lat-cache-miss, Model: Random Forest, Accuracy: 0.9600, F1-Score: 0.9100
  Counter: br-misp-retired-all-branches, Model: SVM, Accuracy: 0.7889, F1-Score: 0.0000
  Counter: br-misp-retired-all-branches, Model: Decision Tree, Accuracy: 0.9756, F1-Score: 0.9399
  Counter: br-misp-retired-all-branches, Model: Random Forest, Accuracy: 0.9756, F1-Score: 0.9399
  Counter: br-inst-retired-all-branches, Model: SVM, Accuracy: 0.7889, F1-Score: 0.0000
  Counter: br-inst-retired-all-branches, Model: Decision Tree, Accuracy: 0.9489, F1-Score: 0.8783
  Counter: br-inst-retired-all-branches, Model: Random Forest, Accuracy: 0.9489, F1-Score: 0.8783
  Counter: cycle-activity-stalls-total, Model: SVM, Accuracy: 0.9600, F1-Score: 0.9135
  Counter: cycle-activity-stalls-total, Model: Decision Tree, Accuracy: 0.9733, F1-Score: 0.9375
  Counter: cycle-activity-stalls-total, Model: Random Forest, Accuracy: 0.9733, F1-Score: 0.9375
  Counter: cache-misses, Model: SVM, Accuracy: 0.7889, F1-Score: 0.0000
  Counter: cache-misses, Model: Decision Tree, Accuracy: 0.9511, F1-Score: 0.8842
  Counter: cache-misses, Model: Random Forest, Accuracy: 0.9511, F1-Score: 0.8842
  Counter: L1-icache-load-misses, Model: SVM, Accuracy: 0.8080, F1-Score: 0.0000
  Counter: L1-icache-load-misses, Model: Decision Tree, Accuracy: 0.7433, F1-Score: 0.4103
  Counter: L1-icache-load-misses, Model: Random Forest, Accuracy: 0.7433, F1-Score: 0.4103
  Counter: machine-clears-smc, Model: SVM, Accuracy: 0.9844, F1-Score: 0.9645
  Counter: machine-clears-smc, Model: Decision Tree, Accuracy: 1.0000, F1-Score: 1.0000
  Counter: machine-clears-smc, Model: Random Forest, Accuracy: 1.0000, F1-Score: 1.0000
  Counter: machine-clears-count, Model: SVM, Accuracy: 0.9178, F1-Score: 0.8063
  Counter: machine-clears-count, Model: Decision Tree, Accuracy: 0.9333, F1-Score: 0.8352
  Counter: machine-clears-count, Model: Random Forest, Accuracy: 0.9333, F1-Score: 0.8352
  Counter: cache-references, Model: SVM, Accuracy: 0.7889, F1-Score: 0.0000
  Counter: cache-references, Model: Decision Tree, Accuracy: 0.9067, F1-Score: 0.7789
  Counter: cache-references, Model: Random Forest, Accuracy: 0.9067, F1-Score: 0.7789

=== Scenario 3 Benign & PNiP + iSpectre ===
  Counter: longest-lat-cache-miss, Model: SVM, Accuracy: 0.8656, F1-Score: 0.8111
  Counter: longest-lat-cache-miss, Model: Decision Tree, Accuracy: 0.8996, F1-Score: 0.8549
  Counter: longest-lat-cache-miss, Model: Random Forest, Accuracy: 0.8996, F1-Score: 0.8549
  Counter: br-misp-retired-all-branches, Model: SVM, Accuracy: 0.6523, F1-Score: 0.0000
  Counter: br-misp-retired-all-branches, Model: Decision Tree, Accuracy: 0.9337, F1-Score: 0.9034
  Counter: br-misp-retired-all-branches, Model: Random Forest, Accuracy: 0.9337, F1-Score: 0.9034
  Counter: br-inst-retired-all-branches, Model: SVM, Accuracy: 0.6523, F1-Score: 0.0000
  Counter: br-inst-retired-all-branches, Model: Decision Tree, Accuracy: 0.8978, F1-Score: 0.8519
  Counter: br-inst-retired-all-branches, Model: Random Forest, Accuracy: 0.8978, F1-Score: 0.8519
  Counter: cycle-activity-stalls-total, Model: SVM, Accuracy: 0.9140, F1-Score: 0.8899
  Counter: cycle-activity-stalls-total, Model: Decision Tree, Accuracy: 0.9498, F1-Score: 0.9286
  Counter: cycle-activity-stalls-total, Model: Random Forest, Accuracy: 0.9498, F1-Score: 0.9286
  Counter: cache-misses, Model: SVM, Accuracy: 0.7867, F1-Score: 0.6338
  Counter: cache-misses, Model: Decision Tree, Accuracy: 0.8925, F1-Score: 0.8454
  Counter: cache-misses, Model: Random Forest, Accuracy: 0.8925, F1-Score: 0.8454
  Counter: L1-icache-load-misses, Model: SVM, Accuracy: 0.7194, F1-Score: 0.5491
  Counter: L1-icache-load-misses, Model: Decision Tree, Accuracy: 0.6888, F1-Score: 0.5642
  Counter: L1-icache-load-misses, Model: Random Forest, Accuracy: 0.6888, F1-Score: 0.5642
  Counter: machine-clears-smc, Model: SVM, Accuracy: 0.8405, F1-Score: 0.7023
  Counter: machine-clears-smc, Model: Decision Tree, Accuracy: 0.9857, F1-Score: 0.9792
  Counter: machine-clears-smc, Model: Random Forest, Accuracy: 0.9857, F1-Score: 0.9792
  Counter: machine-clears-count, Model: SVM, Accuracy: 0.9283, F1-Score: 0.8974
  Counter: machine-clears-count, Model: Decision Tree, Accuracy: 0.9265, F1-Score: 0.8941
  Counter: machine-clears-count, Model: Random Forest, Accuracy: 0.9283, F1-Score: 0.8969
  Counter: cache-references, Model: SVM, Accuracy: 0.6523, F1-Score: 0.0000
  Counter: cache-references, Model: Decision Tree, Accuracy: 0.8835, F1-Score: 0.8276
  Counter: cache-references, Model: Random Forest, Accuracy: 0.8835, F1-Score: 0.8276
\end{comment}



\begin{comment}
    === Scenario 1 Benign & PNiP ===
  Counter: cache-references, Model: SVM, Accuracy: 0.8008, F1-Score: 0.0000
  Counter: cache-references, Model: Decision Tree, Accuracy: 0.9023, F1-Score: 0.7536
  Counter: cache-references, Model: Random Forest, Accuracy: 0.9023, F1-Score: 0.7536
  Counter: br-misp-retired-all-branches, Model: SVM, Accuracy: 0.8008, F1-Score: 0.0000
  Counter: br-misp-retired-all-branches, Model: Decision Tree, Accuracy: 0.9195, F1-Score: 0.7981
  Counter: br-misp-retired-all-branches, Model: Random Forest, Accuracy: 0.9195, F1-Score: 0.7981
  Counter: L1-icache-load-misses, Model: SVM, Accuracy: 0.8697, F1-Score: 0.7490
  Counter: L1-icache-load-misses, Model: Decision Tree, Accuracy: 0.8761, F1-Score: 0.7157
  Counter: L1-icache-load-misses, Model: Random Forest, Accuracy: 0.8739, F1-Score: 0.7122
  Counter: machine-clears-count, Model: SVM, Accuracy: 0.9904, F1-Score: 0.9758
  Counter: machine-clears-count, Model: Decision Tree, Accuracy: 0.9981, F1-Score: 0.9952
  Counter: machine-clears-count, Model: Random Forest, Accuracy: 0.9981, F1-Score: 0.9952
  Counter: cycle-activity-stalls-total, Model: SVM, Accuracy: 0.7931, F1-Score: 0.0690
  Counter: cycle-activity-stalls-total, Model: Decision Tree, Accuracy: 0.9655, F1-Score: 0.9182
  Counter: cycle-activity-stalls-total, Model: Random Forest, Accuracy: 0.9655, F1-Score: 0.9182
  Counter: cache-misses, Model: SVM, Accuracy: 0.8008, F1-Score: 0.0000
  Counter: cache-misses, Model: Decision Tree, Accuracy: 0.9023, F1-Score: 0.7512
  Counter: cache-misses, Model: Random Forest, Accuracy: 0.9023, F1-Score: 0.7512
  Counter: machine-clears-smc, Model: SVM, Accuracy: 0.9943, F1-Score: 0.9854
  Counter: machine-clears-smc, Model: Decision Tree, Accuracy: 0.9943, F1-Score: 0.9854
  Counter: machine-clears-smc, Model: Random Forest, Accuracy: 0.9943, F1-Score: 0.9854
  Counter: br-inst-retired-all-branches, Model: SVM, Accuracy: 0.8008, F1-Score: 0.0000
  Counter: br-inst-retired-all-branches, Model: Decision Tree, Accuracy: 0.8946, F1-Score: 0.7317
  Counter: br-inst-retired-all-branches, Model: Random Forest, Accuracy: 0.8946, F1-Score: 0.7317
  Counter: longest-lat-cache-miss, Model: SVM, Accuracy: 0.7897, F1-Score: 0.0000
  Counter: longest-lat-cache-miss, Model: Decision Tree, Accuracy: 0.8889, F1-Score: 0.7282
  Counter: longest-lat-cache-miss, Model: Random Forest, Accuracy: 0.8889, F1-Score: 0.7282

=== Scenario 2 Benign & iSpectre ===
  Counter: cache-references, Model: SVM, Accuracy: 0.8008, F1-Score: 0.0000
  Counter: cache-references, Model: Decision Tree, Accuracy: 0.8946, F1-Score: 0.7343
  Counter: cache-references, Model: Random Forest, Accuracy: 0.8946, F1-Score: 0.7343
  Counter: br-misp-retired-all-branches, Model: SVM, Accuracy: 0.8008, F1-Score: 0.0000
  Counter: br-misp-retired-all-branches, Model: Decision Tree, Accuracy: 0.9598, F1-Score: 0.8986
  Counter: br-misp-retired-all-branches, Model: Random Forest, Accuracy: 0.9598, F1-Score: 0.8986
  Counter: L1-icache-load-misses, Model: SVM, Accuracy: 0.7842, F1-Score: 0.0000
  Counter: L1-icache-load-misses, Model: Decision Tree, Accuracy: 0.7308, F1-Score: 0.4057
  Counter: L1-icache-load-misses, Model: Random Forest, Accuracy: 0.7308, F1-Score: 0.4057
  Counter: machine-clears-count, Model: SVM, Accuracy: 0.8927, F1-Score: 0.7143
  Counter: machine-clears-count, Model: Decision Tree, Accuracy: 0.9234, F1-Score: 0.8077
  Counter: machine-clears-count, Model: Random Forest, Accuracy: 0.9234, F1-Score: 0.8077
  Counter: cycle-activity-stalls-total, Model: SVM, Accuracy: 0.9540, F1-Score: 0.8966
  Counter: cycle-activity-stalls-total, Model: Decision Tree, Accuracy: 0.9847, F1-Score: 0.9623
  Counter: cycle-activity-stalls-total, Model: Random Forest, Accuracy: 0.9847, F1-Score: 0.9623
  Counter: cache-misses, Model: SVM, Accuracy: 0.8008, F1-Score: 0.0000
  Counter: cache-misses, Model: Decision Tree, Accuracy: 0.9598, F1-Score: 0.8995
  Counter: cache-misses, Model: Random Forest, Accuracy: 0.9598, F1-Score: 0.8995
  Counter: machine-clears-smc, Model: SVM, Accuracy: 0.9866, F1-Score: 0.9674
  Counter: machine-clears-smc, Model: Decision Tree, Accuracy: 1.0000, F1-Score: 1.0000
  Counter: machine-clears-smc, Model: Random Forest, Accuracy: 1.0000, F1-Score: 1.0000
  Counter: br-inst-retired-all-branches, Model: SVM, Accuracy: 0.8008, F1-Score: 0.0000
  Counter: br-inst-retired-all-branches, Model: Decision Tree, Accuracy: 0.9464, F1-Score: 0.8641
  Counter: br-inst-retired-all-branches, Model: Random Forest, Accuracy: 0.9464, F1-Score: 0.8641
  Counter: longest-lat-cache-miss, Model: SVM, Accuracy: 0.7897, F1-Score: 0.0000
  Counter: longest-lat-cache-miss, Model: Decision Tree, Accuracy: 0.9663, F1-Score: 0.9209
  Counter: longest-lat-cache-miss, Model: Random Forest, Accuracy: 0.9663, F1-Score: 0.9209

=== Scenario 3 Benign & PNiP + iSpectre ===
  Counter: cache-references, Model: SVM, Accuracy: 0.6746, F1-Score: 0.0000
  Counter: cache-references, Model: Decision Tree, Accuracy: 0.8492, F1-Score: 0.7786
  Counter: cache-references, Model: Random Forest, Accuracy: 0.8492, F1-Score: 0.7786
  Counter: br-misp-retired-all-branches, Model: SVM, Accuracy: 0.6746, F1-Score: 0.0000
  Counter: br-misp-retired-all-branches, Model: Decision Tree, Accuracy: 0.9206, F1-Score: 0.8768
  Counter: br-misp-retired-all-branches, Model: Random Forest, Accuracy: 0.9206, F1-Score: 0.8768
  Counter: L1-icache-load-misses, Model: SVM, Accuracy: 0.6962, F1-Score: 0.5179
  Counter: L1-icache-load-misses, Model: Decision Tree, Accuracy: 0.7049, F1-Score: 0.6083
  Counter: L1-icache-load-misses, Model: Random Forest, Accuracy: 0.7049, F1-Score: 0.6083
  Counter: machine-clears-count, Model: SVM, Accuracy: 0.9000, F1-Score: 0.8437
  Counter: machine-clears-count, Model: Decision Tree, Accuracy: 0.9254, F1-Score: 0.8884
  Counter: machine-clears-count, Model: Random Forest, Accuracy: 0.9238, F1-Score: 0.8863
  Counter: cycle-activity-stalls-total, Model: SVM, Accuracy: 0.8968, F1-Score: 0.8632
  Counter: cycle-activity-stalls-total, Model: Decision Tree, Accuracy: 0.9524, F1-Score: 0.9286
  Counter: cycle-activity-stalls-total, Model: Random Forest, Accuracy: 0.9524, F1-Score: 0.9286
  Counter: cache-misses, Model: SVM, Accuracy: 0.6730, F1-Score: 0.0000
  Counter: cache-misses, Model: Decision Tree, Accuracy: 0.8889, F1-Score: 0.8293
  Counter: cache-misses, Model: Random Forest, Accuracy: 0.8889, F1-Score: 0.8293
  Counter: machine-clears-smc, Model: SVM, Accuracy: 0.8429, F1-Score: 0.6817
  Counter: machine-clears-smc, Model: Decision Tree, Accuracy: 0.9984, F1-Score: 0.9976
  Counter: machine-clears-smc, Model: Random Forest, Accuracy: 0.9984, F1-Score: 0.9976
  Counter: br-inst-retired-all-branches, Model: SVM, Accuracy: 0.6746, F1-Score: 0.0000
  Counter: br-inst-retired-all-branches, Model: Decision Tree, Accuracy: 0.8889, F1-Score: 0.8276
  Counter: br-inst-retired-all-branches, Model: Random Forest, Accuracy: 0.8889, F1-Score: 0.8276
  Counter: longest-lat-cache-miss, Model: SVM, Accuracy: 0.6503, F1-Score: 0.0000
  Counter: longest-lat-cache-miss, Model: Decision Tree, Accuracy: 0.9101, F1-Score: 0.8712
  Counter: longest-lat-cache-miss, Model: Random Forest, Accuracy: 0.9101, F1-Score: 0.8712
\end{comment}
